# Supplementary material for: PixelLM: Pixel Reasoning with Large Multimodal Model
Source: arXiv:2312.02228 source file (2024-07-18)
Supplement: Supplementary file 1 [file X_suppl_old.tex]

\clearpage
\newpage
\appendix
\maketitlesupplementary

\renewcommand\thefigure{\thesection.\arabic{figure}}
\renewcommand\thetable{\thesection.\arabic{table}}
\setcounter{figure}{0} 
\setcounter{table}{0} 
\setcounter{table}{0}
\renewcommand{\thetable}{A.\arabic{table}}

\section*{Appendix}
In this supplementary material, we first detail the training configuration, decoder structure, flops calculation, and MUSE evaluation process in Sec.~\ref{sec:supp_implement}. We then present additional experimental analysis of our segmentation codebook and decoder in Sec.~\ref{sec:supp_exp}. We further offer a more comprehensive analysis of MUSE and the multi-referring segmentation dataset in Sec.~\ref{sec:sup_muse} 
% \XJ{also mention the multi-referring seg. dataset since it is important}. 

\section{Implementation Details}
\label{sec:supp_implement}
\noindent \textbf{Training detail.} 
We give the detailed training configuration in Tab.~\ref{table:supp_training_setting}, we do \textit{not} use color jittering, drop path or gradient clip. The gradient accumulation step is set to 10.

\noindent \textbf{Structure detail of decoder.} 
\ZW{We now elaborate on our decoder structure in detail. The decoder's function is divided into three parts: \textit{i}) the attention block for each scale; \textit{ii}) updating the features of the next scale using the output of the previous scale's attention block; \textit{iii}) fusion of the final results. Each part and their combination are presented in Alg.~\ref{alg:code}, styled similarly to PyTorch code.}
% Alg.~\ref{alg:code} provides the pseudo-code of our pixel decoder in a PyTorch-like style.

\XJ{For clarity, we should also add some explanations to the structure and refer the explanation to the figure in main text. Only placing pseudo code here may not help much the understanding of the decoder.}

\XJ{Besides, the Alg.1 should be reorganized to be more structured for clarity. We may first split the codes into major groups according to their functions, then use 1, 2, 3.. followed by brief intro. of their functions as comments in the begginig of each group.   }


\noindent \textbf{Calculation of TFLOPs.} \XJ{may need to also explain the T in TFLOPs. Explain exactly the same term TFLOPs as shown in table} We calculate the TFlops (\ZW{a unit of computing speed equal to one trillion  floating-point operations per second}) of our models in Tab.~\ref{table:reason_seg}. We refer to the formula provided in \cite{clark2020electra} and the script from DeepSpeed~\cite{deepspeed} for the calculation. Since the flops for LMMs vary with the generated token length, we set the token length of our LMM at 512, which is a common default length used by~\cite{liu2023llava,touvron2023llama} and also can accommodate dozens of target objects. 
% \XJ{why use this length? does it has any special meaning, like it is a typical length of output? or the average length we calculate for some set of examples.}, accommodating dozens of target objects. 
% The primary computational burden arises from the transformer blocks, and the calculation formula is as follows:


\noindent \textbf{Details of the evaluation metric.}
Section~\ref{subsec:evaluation} provides a concise overview of the MUSE 
% \XJ{we never use ``multi-reasoning segmentation" in the main text, do not invent new term or randomly any un-mentioned terms. Use consistent terms throughout the paper.} 
evaluation pipeline. In this sections, we delve into a more formal and detailed explanation of its design. Let us denote by $M=\{M_g\}_{g=1}^G$ the ground truth set of $G$ objects, and $\hat{M}=\{\hat{M_k}\}_{k=1}^K$ the set of $K$ predictions. Motivated by ~\cite{detr}, assuming $K$ is not equal to $G$, we use $\varnothing$ (no objects) to pad the smaller set and both sets finally have size $N={\rm max}(G, K)$. To find a bipartite matching between these two sets we search for a permutation of $N$
elements $\sigma\in\mathfrak{S}_N$ with the lowest cost:
\begin{equation}
    \hat{\sigma} = \mathop{\arg\min}\limits_{\sigma\in\mathfrak{S}_N} \sum_{i}^{N} \mathcal{L}_{match}(M_i, \hat{M}_{\sigma(i)})  
\end{equation}
where $\mathcal{L}_{match}(M_i, \hat{M}_{\sigma(i)})$ is a pair-wise matching cost between ground truth $M_i$ and a prediction with index $\sigma(i)$. This optimal assignment is computed efficiently
with the Hungarian algorithm. We define $\mathcal{L}_{match}(M_i, \hat{M}_{\sigma(i)})$ as $\mathcal{L}_{bce}(M_i, \hat{M}_{\sigma(i)}) + \mathcal{L}_{dice}(M_i, \hat{M}_{\sigma(i)})$.

Based on the matching results, we modify the generated response $y_{res}$ to $y_{res}^{\prime}$: since each $\hat{M}_i$ originates from a segmentation token sequence in $y_{res}$, we replace each sequence with the GPT-generated description of $M_i$. Subsequently, we employ a carefully designed prompt for GPT-3.5 to give a score $s_i$ to each $\hat{M}_i$. An example of this methodology is depicted in Fig.~\ref{fig:supp_evaluation}. The empty predictions are directly scored with 0. The final IoU of each prediction is:
\begin{equation}
\begin{aligned}
{\rm Intersection}_i &= \left\{ 
    \begin{array}{lc}
        {\rm Intersection}_i &s_i>0.5 \\
        0 &s_i\leq0.5
    \end{array} \right. \\
{\rm IoU}_i &= {\rm Intersection}_i / {\rm Union}_i
\end{aligned} 
\end{equation}
Based on the IoU scores, we can calculate gIoU and cIoU metric like referring segmentation dataset.


\input{table/sup_detail}
\input{table/supp_scale_share}
\input{table/decoder_alg_v3}

\begin{figure*}[t]
\includegraphics[width=1\linewidth]{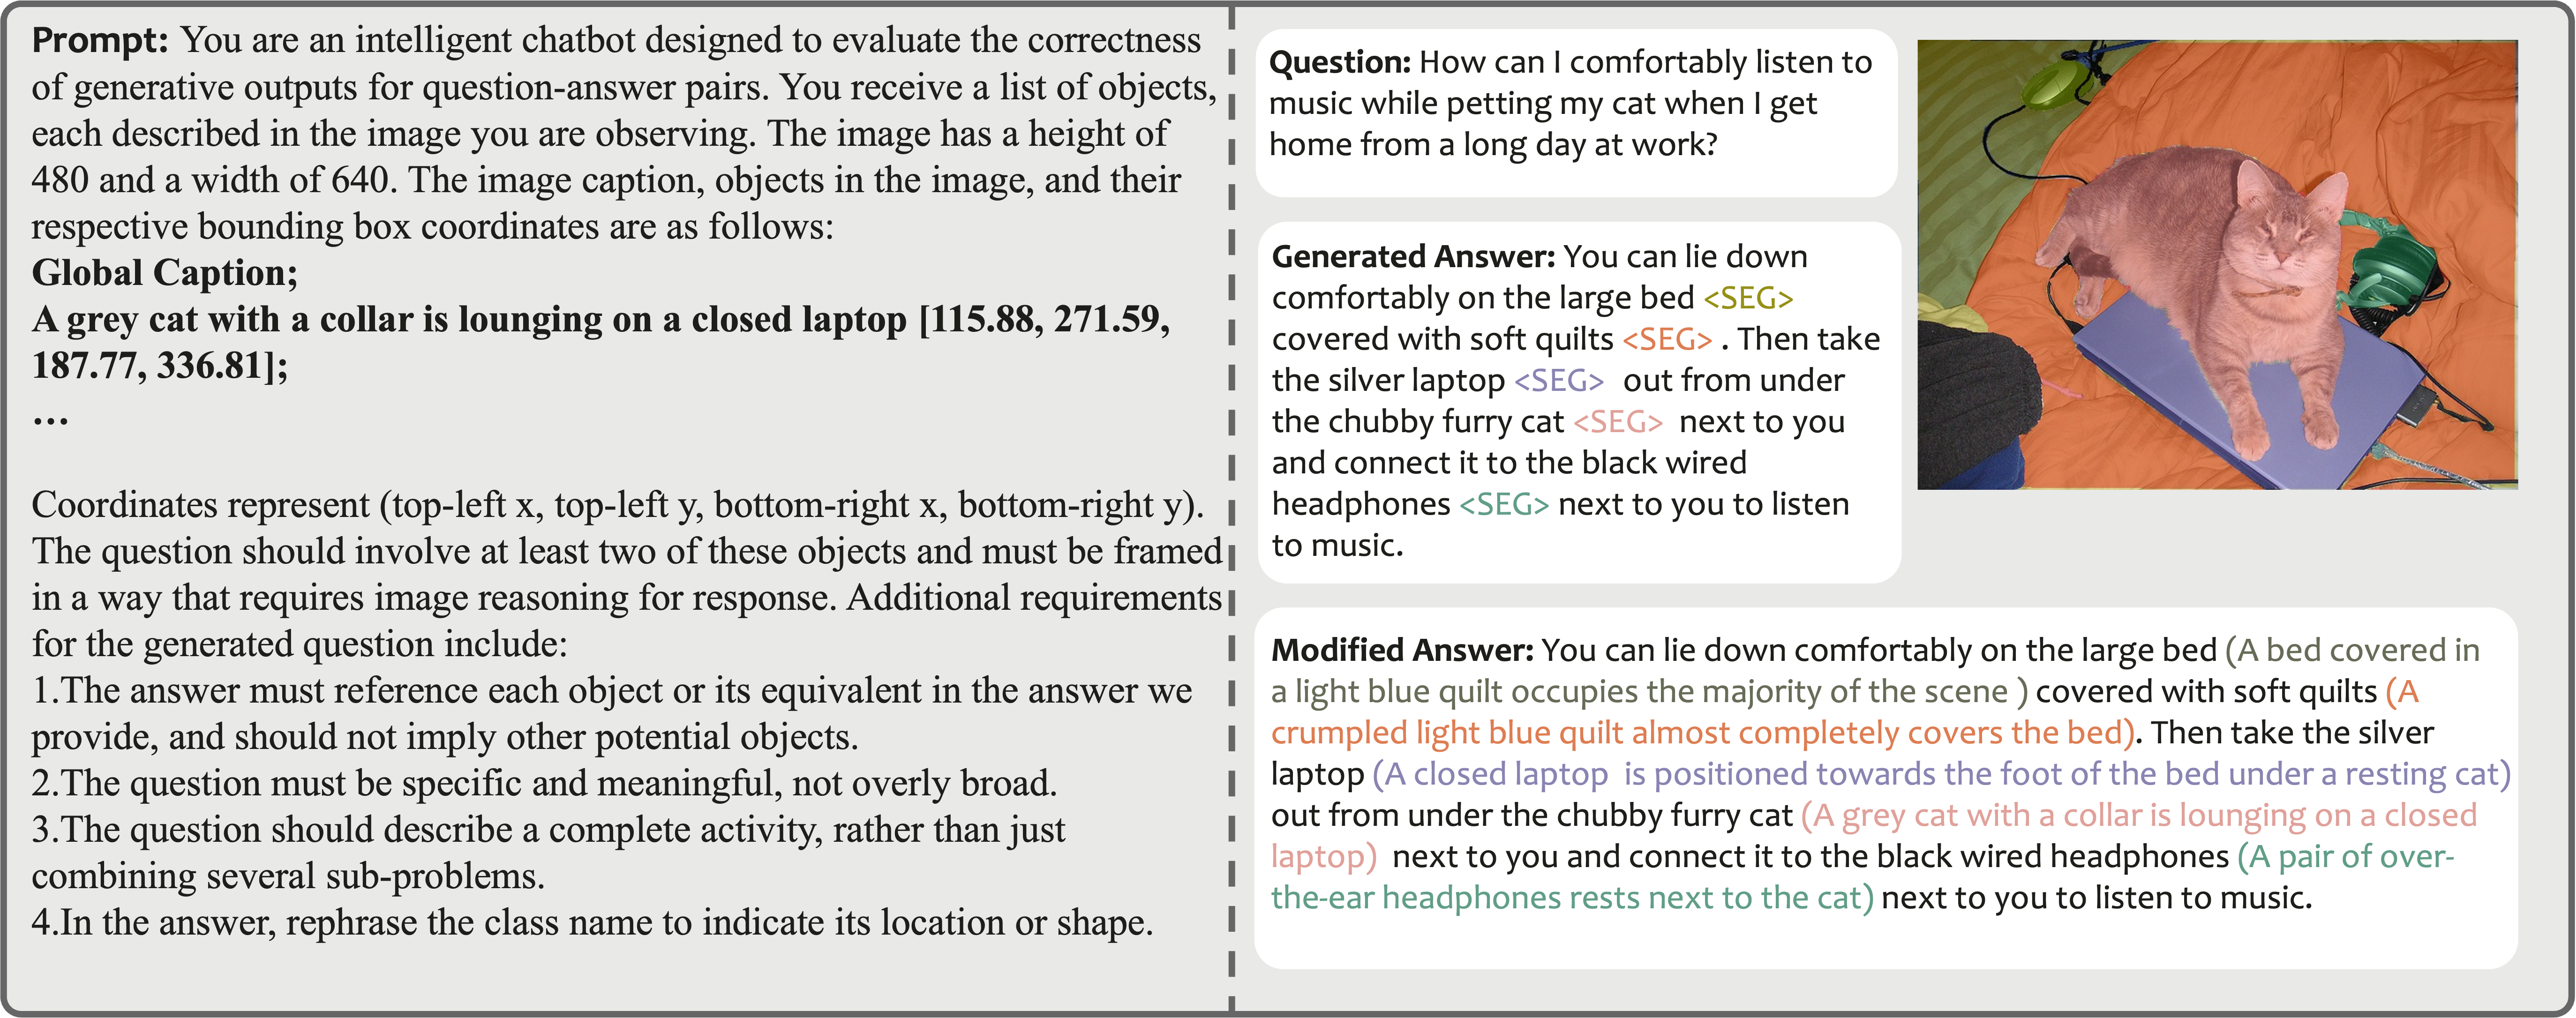}
\centering
\vspace{-3pt}
\caption{\textbf{Evaluation example.} The left panel illustrates the prompt employed in our GPT evaluation pipeline. The right panel showcases an example of a predicted answer alongside its corresponding modified version, as input to GPT.}
\label{fig:supp_evaluation}
\end{figure*}

\begin{figure*}[t]\centering
  \subfloat[\label{fig:cat_number}The number of instances per category]{\includegraphics[width=0.32\linewidth]{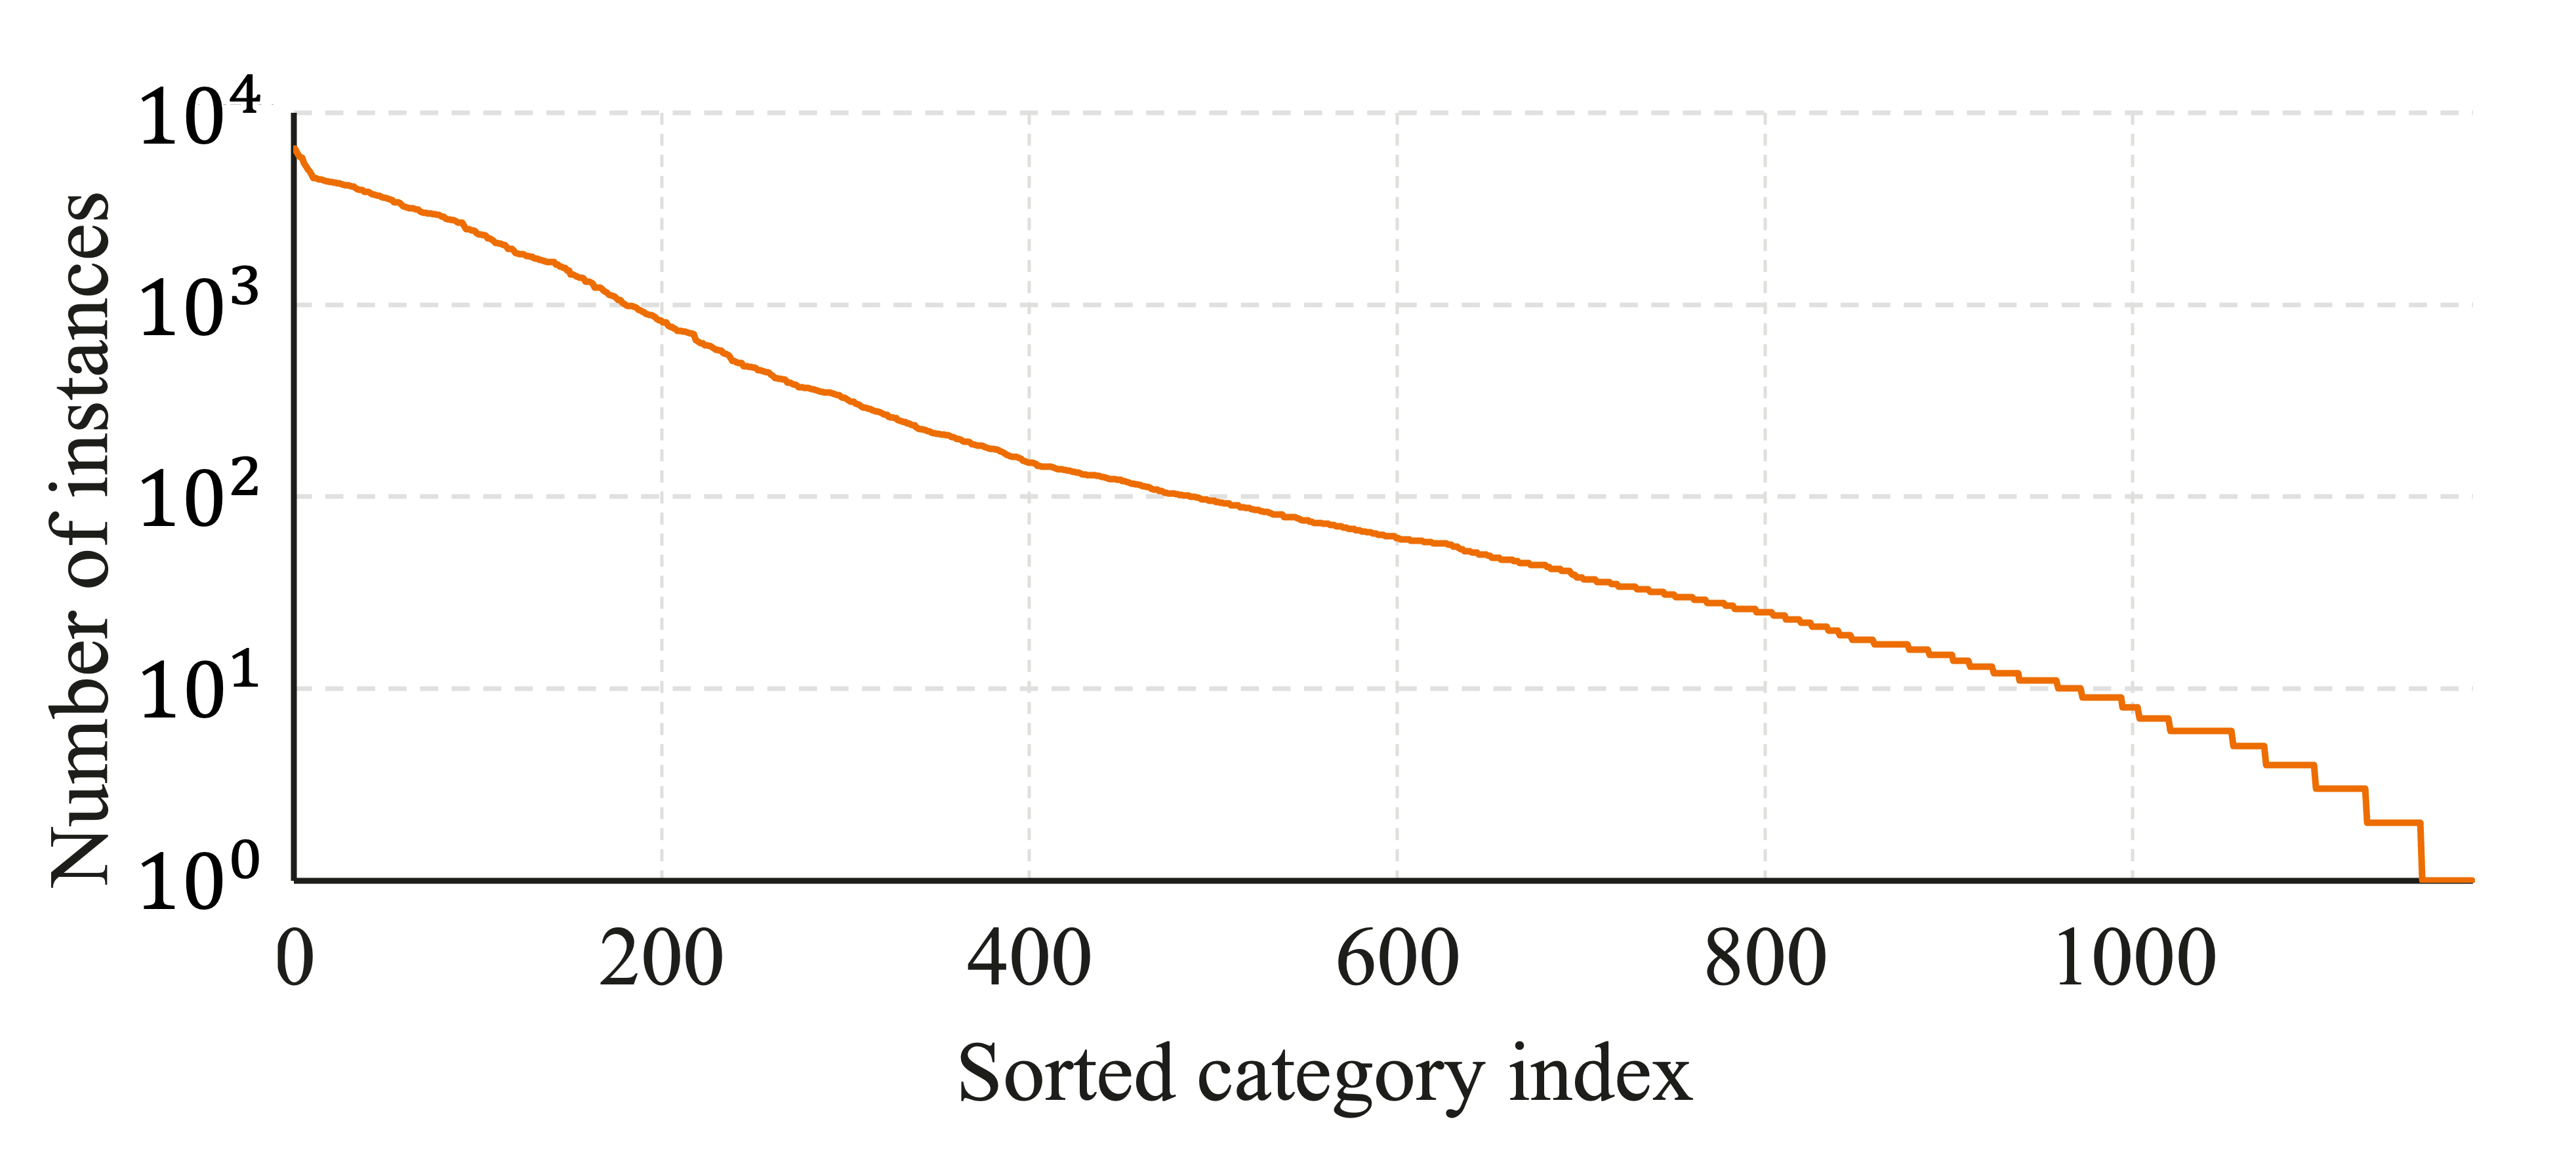}  }
\hfill
\subfloat[\label{fig:token_number}Distribution of token count per instance.]{\includegraphics[width=0.32\linewidth]{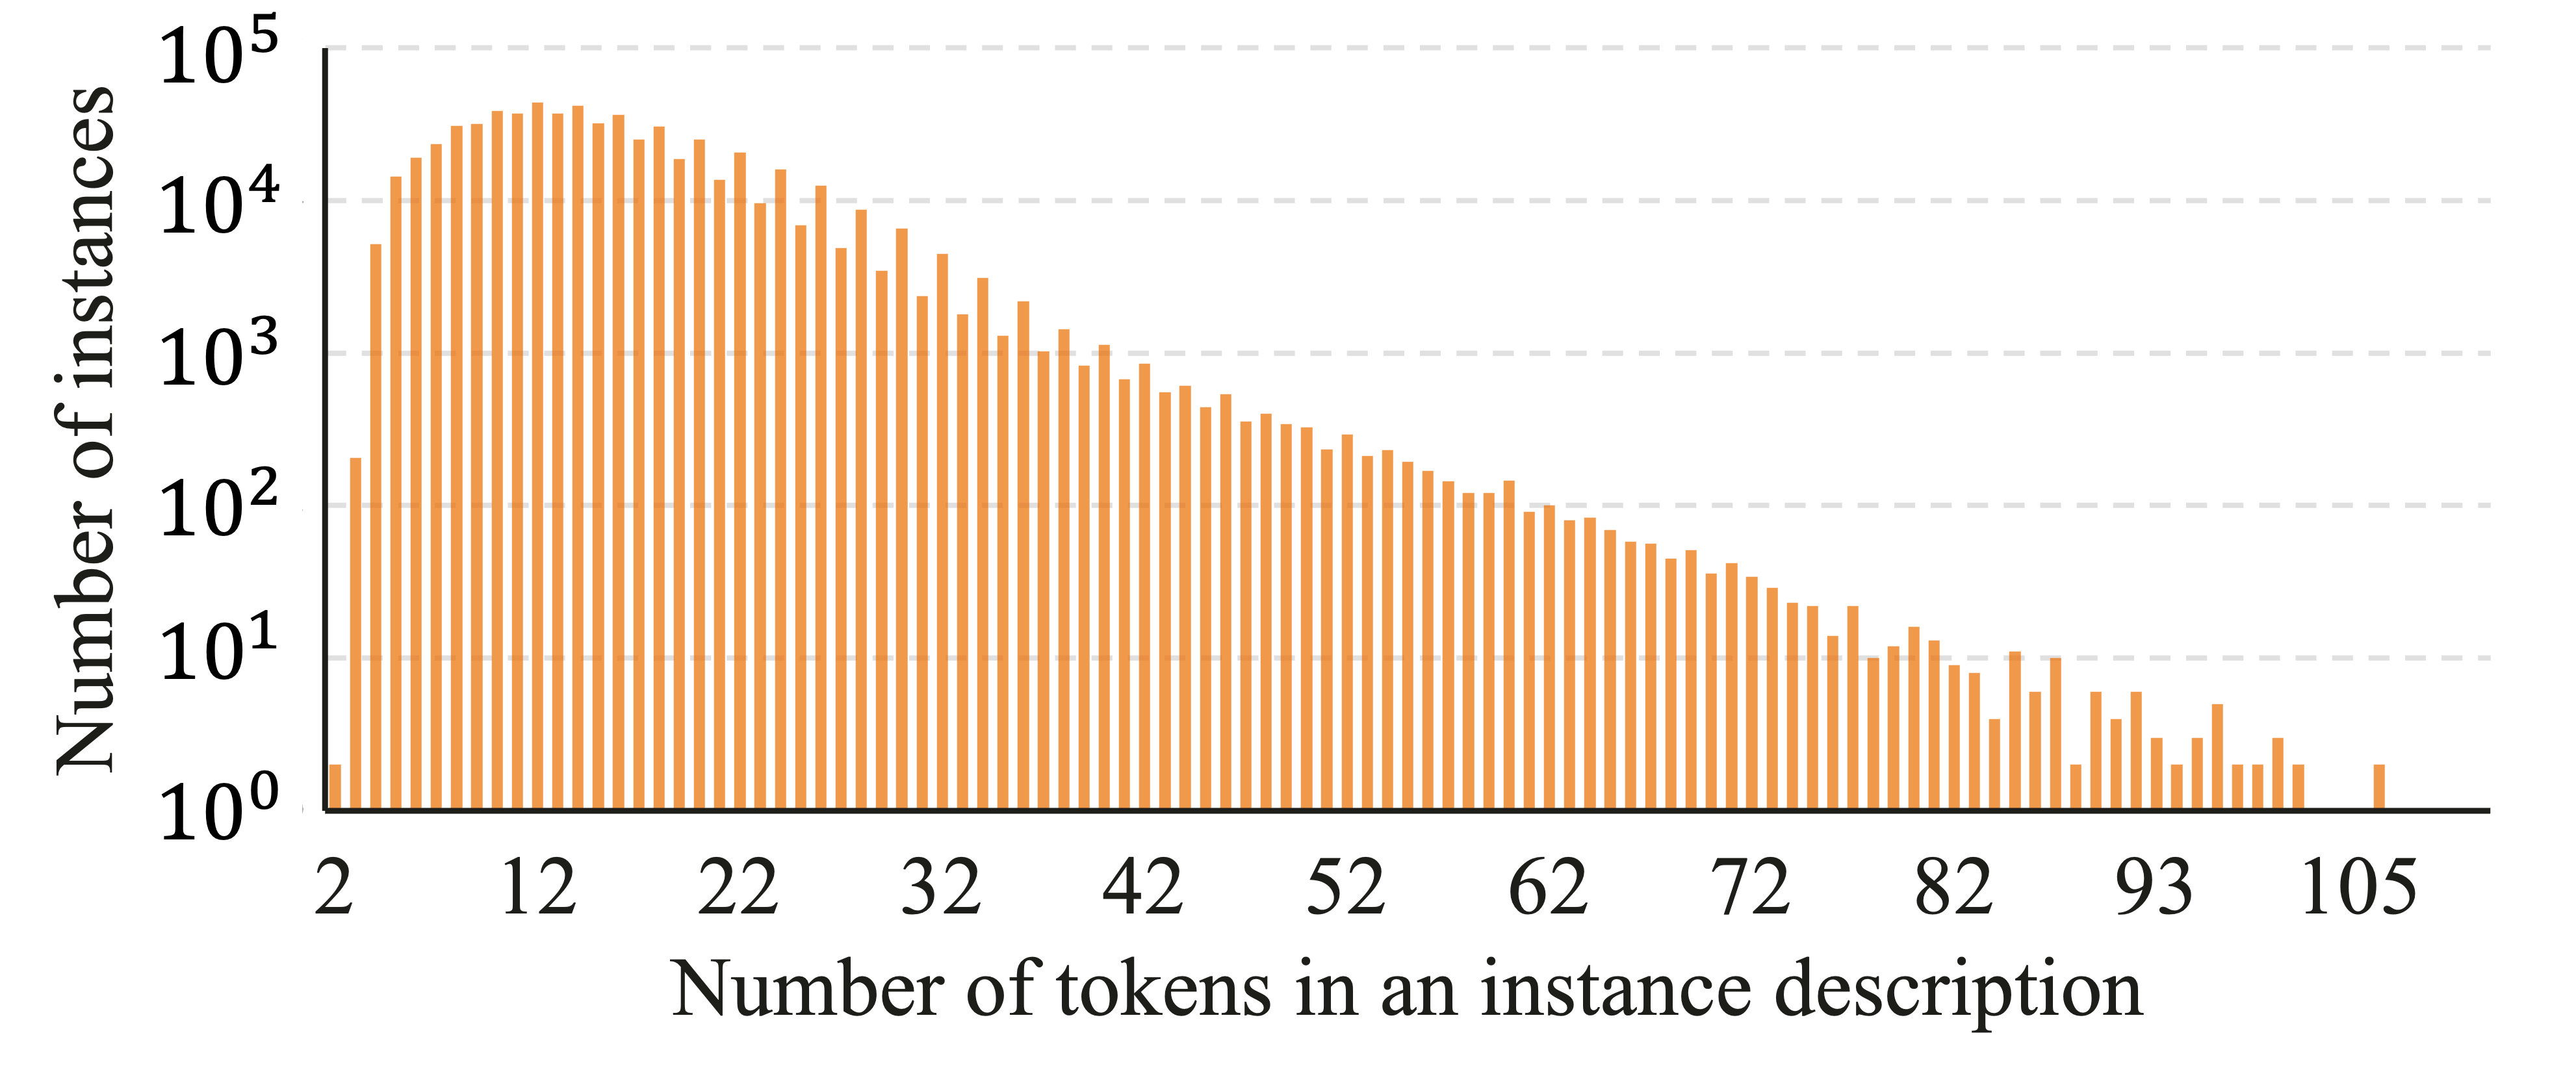} }
\hfill
\subfloat[\label{fig:target_number} Distribution of target count per question.]{\includegraphics[width=0.32\linewidth]{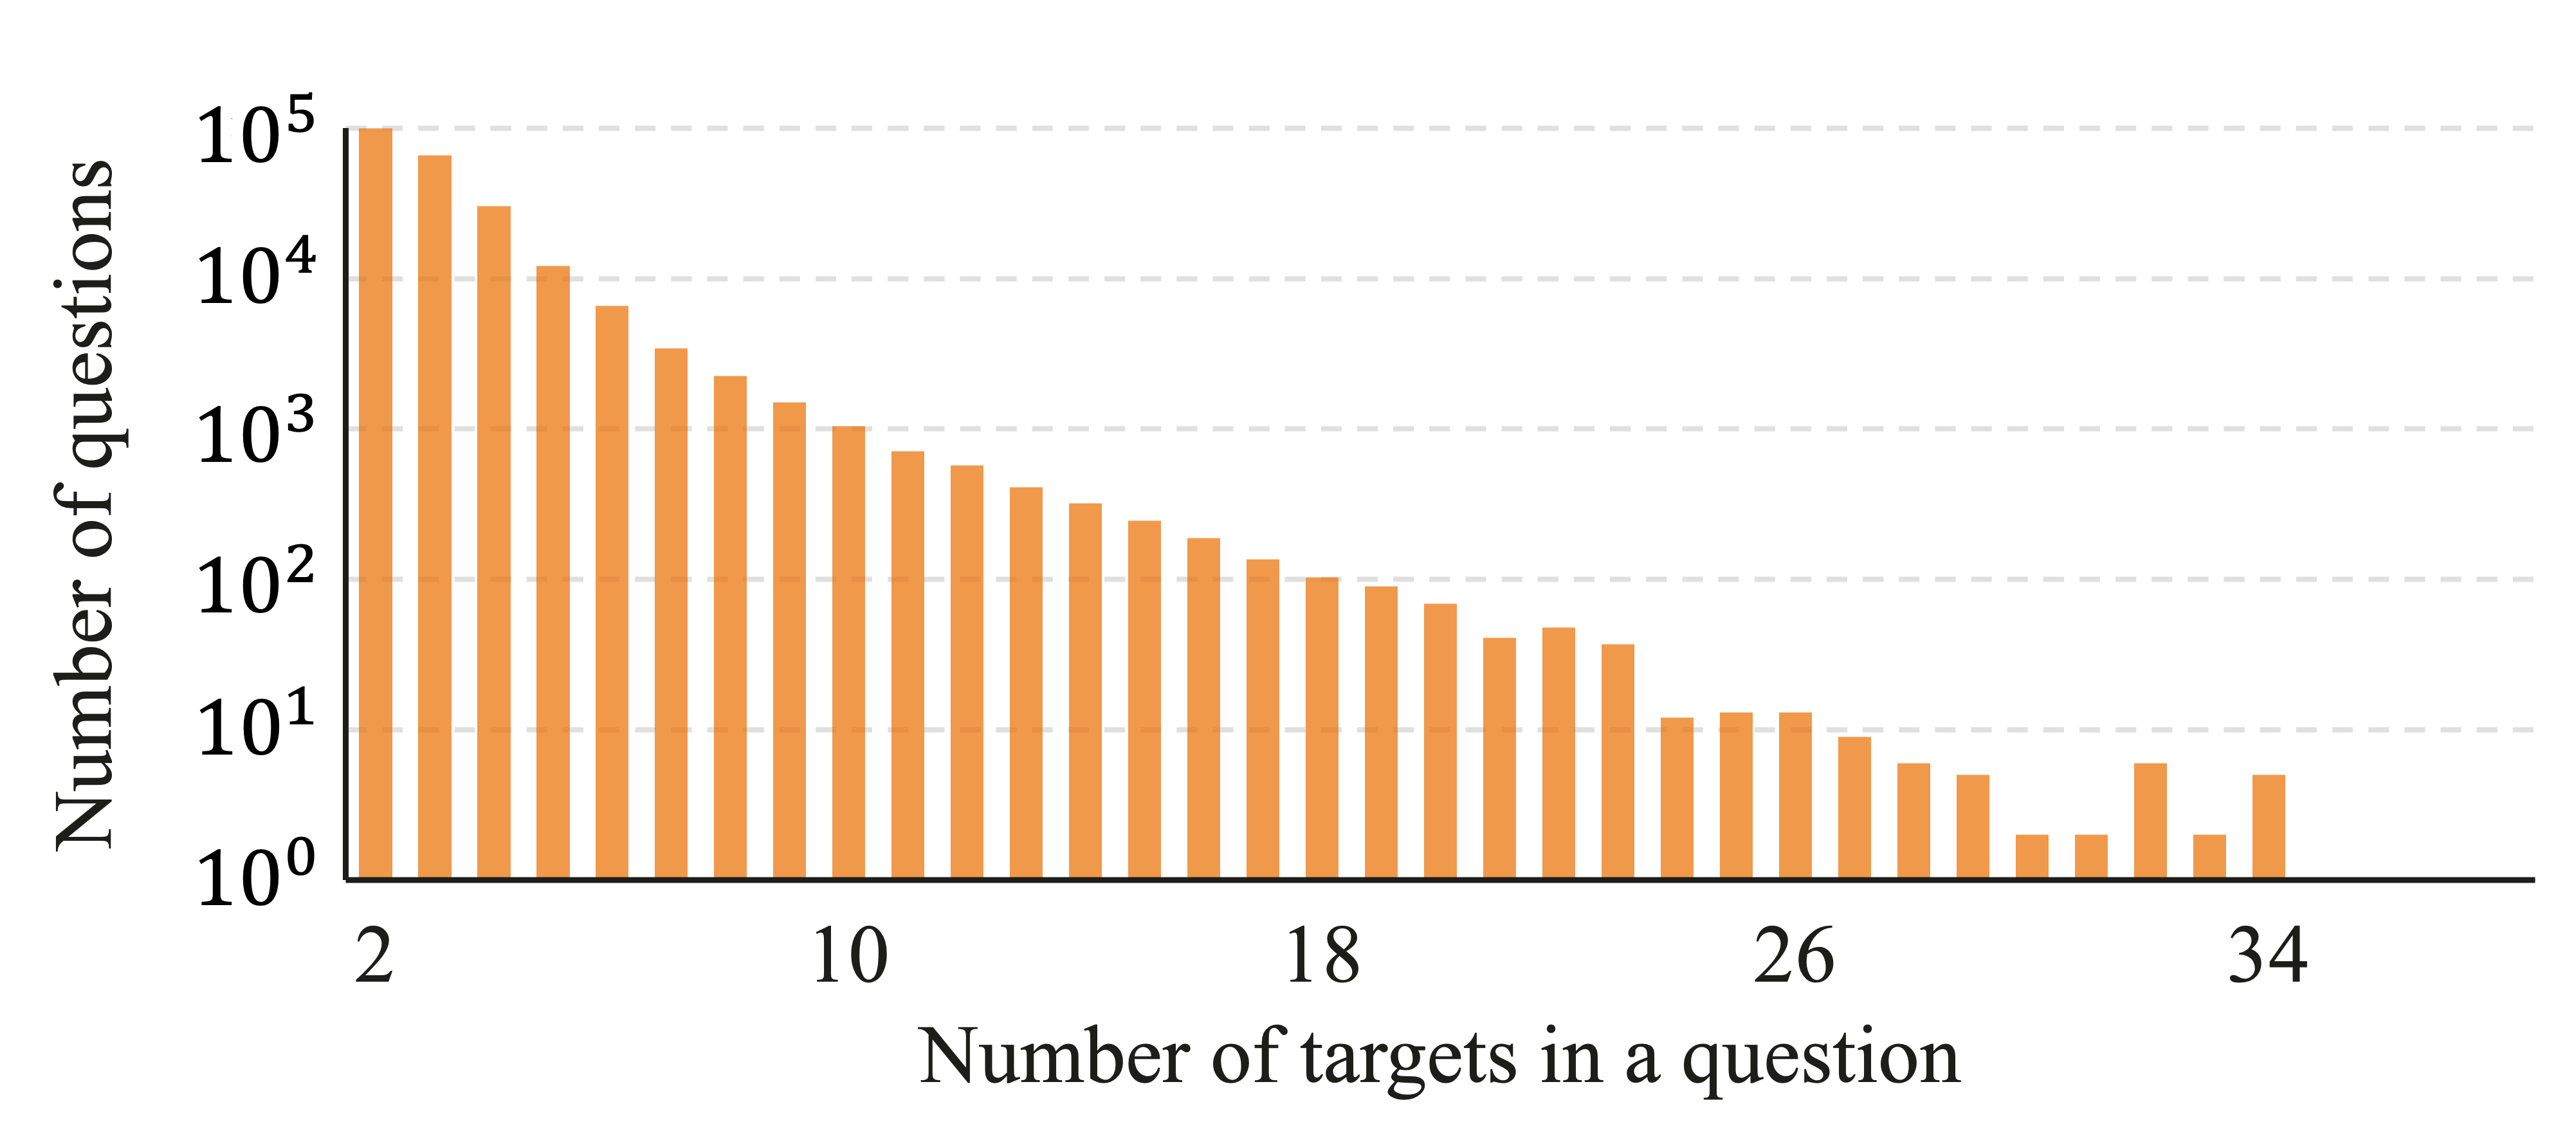}}\\[.25em]
\caption{\textbf{Dataset statistics}. Best viewed digitally.}
\vspace{-3mm}
\label{fig:supp_data_comp}
\end{figure*}

\section{More ablative experiments \XJ{for all titles of section/subsection, always capitalize the first letter of each word. }}
\label{sec:supp_exp}
 
\noindent \textbf{Impact of multi-scale tokens in codebook.} To clearly demonstrate the necessity of our multi-scale segmentation tokens in the codebook $C_{\text{seg}}$, 
\ZW{we still use $L$ multi-scale features, but reduce the original codebook shape of $N\times L$ to $N$, that is the remaining $N$ tokens being identical across $L$ scales.}
\XJ{eliminate dimension is grammarly wrong, simply explaining what we are doing in plain text is fine.} 
As Tab.~\ref{table:supp_scale_share} shows, using a dedicated segmentation token for each scale yields better performance.

\noindent \textbf{Multi-scale layer selection.} \ZW{We experiment with different layer selections in Tab.~\ref{table:supp_scale_selection}. The CLIP-ViT-L used in PixelLM comprises 24 layers. To reduce the computational cost of the decoder, we avoid selecting features from all layers of ViT. Instead, we adhere to the multi-scale feature selection ratio from prior work~\cite{he2015deep,liu2021swin} and explore other selection options. Experiments show that for our task, selecting features from layers before the middle does not offer benefits. Therefore, we mainly focus on selections from the middle and rear layers. The results indicate that using features from 14, 23 layer lead to the best results.} 
 \XJ{briefly explain why ``beyond the midpoint". 
may refer to findings or practices in previous works.}. 
% The results indicate that all selections enhance performance, leading us to choose -2, -11 as our default selection.




\section{More detail about MUSE}
\label{sec:sup_muse}

\subsection{Data filtering}
\noindent \textbf{GPT-4V filtering.} 
\ZW{Although GPT-4V can efficiently understand image content, there are still failure cases in the generated data, and can be summarized as these two points: }
\XJ{what does the limitation mean? should explain briefly. Or do you simply mean following two points? If so, should rephrase this sentence.} 
% in LMMs~\cite{borji2023categorical}, it is necessary to employ a stringent sample filtering process to guarantee the quality of the data. 
% Although GPT-4V can understand image content and follow our instructions very well, failure still arise due to the inherent limitation in LMMs~\cite{borji2023categorical}. 
% In our filtering process, the primary focuses are:
\begin{itemize}
    \item Questions could resulting in vague or multiple interpretations, \eg ``What should I take with me on my outing?'', which is extremely vague because ``outing'' can mean a wide array of activities.
    \item Answers omitting semantically equivalent instances, \eg a question might ask about ``choosing a fruit for a snack'', and the answer may only suggest ``an apple'', ignoring other fruit in the image.
    % \item Questions could resulting in vague or multiple interpretations.
\end{itemize}
Therefore, it is cessary to employ a stringent sample filtering process to guarantee the quality of the data. We develop a GPT-4V assisted data filtering pipeline. This pipeline operates by prompting GPT-4V to evaluate all initial question-answer pairs, based on identified common failure modes. Pairs classified by GPT-4V as falling within these failure categories are removed. This procedure effectively excludes approximately 20\% of the preliminary data. The specific prompts used in this process are detailed in Figure x.
% Therefore, we construct a GPT-4V assisted data filtering pipeline. Specifically, based on the common failure mode, we carefully prompt GPT-4V to give a score to all preliminary question-answer pairs, removing all examples that GPT-4V identify as lying in the failure cases. This process removes about 20\% preliminary data, and the prompts are described in Fig.x

\noindent \textbf{Human verification.} To ensure high quality in the generated question-answer pairs during the evaluation stage, we further engage experienced human annotators to double-check our evaluation set. Our approach is driven by two primary objectives:
% To ensure the high quality of generated question-answer pairs in evaluation stage, we hire experienced human annotators to double-check our evaluation set. We mainly consider two objectives: 
\begin{itemize}
    \item The questions should follow an intuitive and logical sequence that a person would typically think of when viewing the image.
    \item The answers should correspond closely to the way a human would naturally respond to the question
    % \item Questions could resulting in vague or multiple interpretations.
\end{itemize}
\ZW{The above filtering process effectively ensures that the questions in the MUSE dataset are sufficiently challenging for reasoning, and the answers are detailed and accurate.}

\XJ{add a conclusive paragraph here to highlight what are the results/benefits by doing such kinds of filtering.}




\begin{figure*}[t]
\includegraphics[width=1\linewidth]{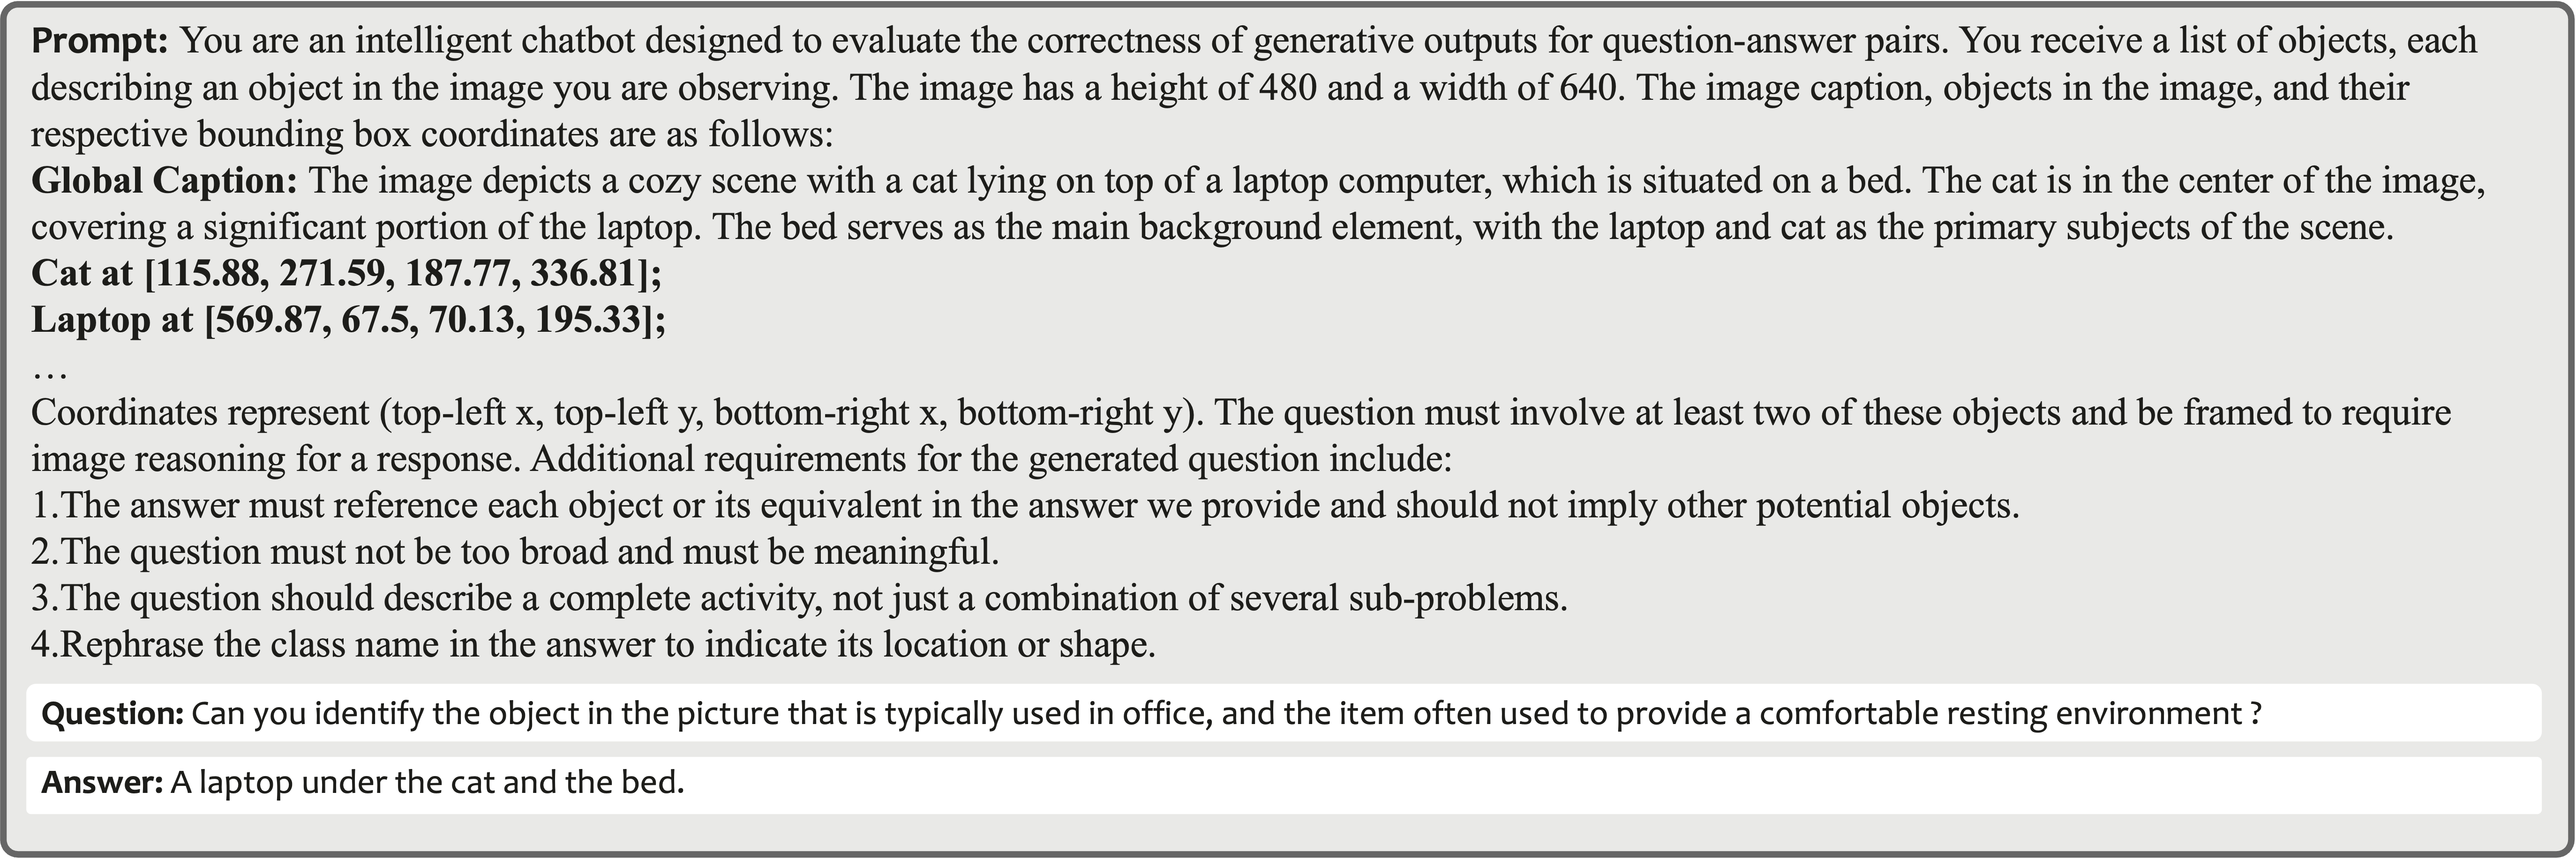}
\centering
\vspace{-3pt}
\caption{\textbf{Example of GPT-4 data generation.} The corresponding image is same as Fig.~\ref{fig:supp_evaluation}.}
\label{fig:supp_gpt4_gen}
\end{figure*}

\subsection{Dataset statistics}
\ZW{In this section, we systematically analyze our dataset. First, our question-answer pairs are based on over 1000 categories, encompassing most objects found in daily scenes. Additionally, the descriptions of objects in the answers are not mere category names limited to a few tokens; they are context-specific descriptions averaging 10 tokens and can extend to over 100 tokens. This proves that our data set covers a very rich object concept, which is very necessary to solve various problems in real scenes.
Finally, we count the number of objects in the answers, covering the range of targets typically involved in reasoning about an image.}

\XJ{the key of introducing statistics is not simply listing all facts, but also use this opportunity to tell others again they are beneficial and why.}
 
\noindent \textbf{Category statistics.} There are over 1000 categories in MUSE from the original LVIS dataset, and 0.9 million instances with unique description that vary based on the context of the question-answer pairs. Fig.~\ref{fig:cat_number} shows the number of instances per category on all question-answer pairs. The distribution inherit the low-shot nature of LVIS.  

\noindent \textbf{Token number statistics.} Fig.~\ref{fig:token_number} displays the instance counts for varying token lengths in the corresponding descriptions. The majority of instances descriptions averaging around 10 tokens, with the highest count reaching an impressive 105 tokens. Although our instances originate from 1023 LVIS categories, they encompass a broader range of semantic concepts after processing through our GPT-4V data generation pipeline. \XJ{above are all just the facts of the dataset, should also briefly highlight the benefits/advantages of these ``facts'' to our concerned tasks or model training.}

\noindent \textbf{Target number statistics.} Fig.~\ref{fig:target_number} presents statistics on the number of targets in each question-answer pair. The average number of targets is 3.7, with the maximum number of targets in a single pair reaching up to 34. \ZW{This number can cover most scenarios of target reasoning for a single image.}
\XJ{similarly, could we add a sentence to connect this statistic number to how we "handle arbitrary number of targets?"}
% Most instances have descriptions of around 10 tokens and the largest tokens-per-instance count is a remarkable 105. Despite our instances are choosen from 1023 categories of LVIS, they can cover many more semantic concepts after processed by our GPT-4V data generation pipeline. 



\subsection{Multi-referring segmentation}
Sec.~\ref{subsec:implement_detail} mentions that we transform vanilla referring segmentation dataset into a multi-referring format for model training. This transformation involves the selection of one to three distinct target objects from the annotations associated with each image. These objects are then used to construct questions in the format: {\tt Please segment the $<$objects$>$ in the image}'', where $<$objects$>$ represents a list of comma-separated object descriptors. 
\ZW{The response format is a list of comma-separated ``{\tt $<$object$>$ is $<$SEG$>$}'', where $<$object$>$ is description of each object.}
\XJ{this symbol $<$SEGs$>$ has never been introduced in the main text so better replace it with another thing to avoid confusion. } 
% for  individual object and ``{\tt $<$objects$>$ are $<$SEGs$>$}'' for multiple objects, with $<$SEGs$>$ denoting a comma-separated list of segmentation token sequences. 
\XJ{we may also need to explain the evaluation of this dataset. this part can be moved to the Evaluation section in supp.}



\subsection{\ZW{More detail about GPT-4 generated data.}}
\XJ{the title of this subsection is not informative. Should be more clear on what this section is about. If it is hard to do so, then do it in the very begining of this subsection. You may begin with things like: ``In this subsection, we $<$summarize the purpose$>$".}
In Sec.~\ref{subsec:ablation}, we create 30,000 additional multi-target question-answer pairs to compare GPT-4 and GPT-4V. The prompts for GPT-4 adhere to similar generation principles but incorporate detailed image captions to offset the absence of visual content. Fig.~\ref{fig:supp_gpt4_gen} demonstrates an example of our GPT-4 data generation process and its typical failures. Given that image content is not directly perceivable, conveying as detailed an image description as possible into GPT-4 is crucial to compensate for this information gap. However, this method often leads to a lack of diversity in the generated question-answer pairs (\ZW{refer to the question-answer pair at the bottom of Fig.~\ref{fig:supp_gpt4_gen}}), characterized by: \XJ{Below points should be supported by concrete examples (maybe examples in the Fig C.3?). Cross-refer to specific places in the figure when writing each point, thus the clarity can be significantly improved.} \textit{i}) Numerous questions are composed of simple referring style sub-questions; \textit{ii}) The question and answer content is limited to what the image caption describes; \textit{iii}) Challenges in generating detailed object descriptions. To address these issues, it might be necessary to introduce more complex annotation details like object relationships, which significantly heightens the complexity of data generation.

% In Sec.~\ref{subsec:ablation}, we create 30,000 additional multi-target question-answer pairs to compare GPT-4 and GPT-4V. The prompts for GPT-4 follow the same generation principles but include detailed image captions to compensate for the lack of visual content. Figure x illustrates an example of our GPT-4 data generation process and its common failures. Since the image content cannot be directly perceived, it is necessary to pass as detailed an image description as possible into GPT-4 to make up for the lack of information. However, this approach still results in a lack of diversity in the generated question-answer pairs: \textit{i}) A large number of questions are spliced into simple referring style sub-questions. 2) The content of the questions and answers cannot exceed what is described in the image caption. 3) It is difficult to generate detailed object descriptions. In order to make up for the above shortcomings, it may be necessary to pass in more complex annotation information such as the relationship between objects, which greatly increases the annotation complexity.
